# Supplementary material for: Equivariant quantizations of the positive nilradical and covariant differential calculi
Source: arXiv:2404.18544 ancillary file (2025-03-28)
Supplement: Supplementary file 1 [file Tensor_product_verification.pdf]

---

## Setting

We consider the simple Lie algebras where a simple root  $\alpha_s$  appears in the highest root with coefficient at least three (these are exactly the exceptional ones).

If  $\alpha_s$  is a simple root as above, we consider a subset of the form  $S = \Pi \setminus \{\alpha_s\}$  together with the grading of the positive roots with respect to  $\alpha_s$ .

Then we consider the simple components  $V_1$  and  $V_3$  of degrees one and three with respect to this grading.

We want to check that the simple component  $V_3$  appears with multiplicity 2 in the tensor product  $V_1^{\otimes 3}$ .

```
In[1]:= << LieART`
```

```
LieART 2.1.0
```

```
last revised 31 March 2022
```

---

## Case $G_2$

```
In[81]:= DynkinDiagram[G2]
```

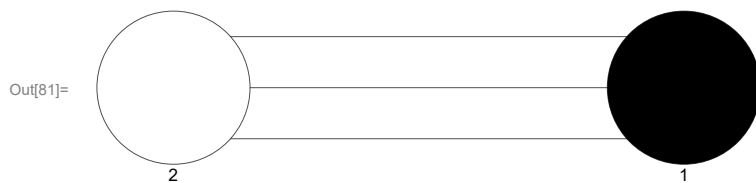

```
In[2]:= AlphaBasis[HighestRoot[G2]]
```

```
Out[2]= (3, 2)
```

```
In[3]:= PositiveRoots[G2]
```

```
Out[3]= { [0 1], [3 -1], [1 0], [-1 1], [-3 2], [2 -1] }
```

```
In[4]:= AlphaBasis[PositiveRoots[G2]]
```

```
Out[4]= {(3, 2), (3, 1), (2, 1), (1, 1), (0, 1), (1, 0)}
```

## Case $\alpha_1$

The semisimple part of the Levi factor is  $A_1$ .

The concrete identification is  $(\alpha_2) \leftrightarrow (\alpha_1)$ .

```
In[5]:= λ[1] = Weight[G2][-1, 1];
```

```
λ[3] = Weight[G2][0, 1];
```

```
In[7]:= AlphaBasis[{λ[1], λ[3]}]
```

```
Out[7]= {(1, 1), (3, 2)}
```

These correspond to the highest weights  $\lambda_1 = \omega_1$  and  $\lambda_3 = \omega_1$ .

```
In[8]:= V[1] = Irrep[A][1];
```

```
In[9]:= DecomposeProduct[V[1], V[1], V[1]] // StandardForm
```

```
Out[9]/StandardForm=
2 (1) + (3)
```

We see that  $V(\omega_1)$  appears with multiplicity two.

## Case $F_4$

```
In[82]:= DynkinDiagram[F4]
```

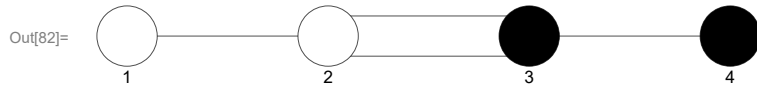

```
In[10]:= AlphaBasis[HighestRoot[F4]]
```

```
Out[10]= (2, 3, 4, 2)
```

```
In[11]:= PositiveRoots[F4]
```

```
Out[11]= {
  {1, 0, 0, 0}, {-1, 1, 0, 0}, {0, -1, 2, 0}, {0, 0, 0, 1}, {0, 0, 1, -1}, {0, 1, -2, 2},
  {0, 1, -1, 0}, {1, -1, 0, 2}, {-1, 0, 0, 2}, {0, 1, 0, -2}, {1, -1, 1, 0}, {-1, 0, 1, 0},
  {1, -1, 2, -2}, {1, 0, -1, 1}, {-1, 0, 2, -2}, {-1, 1, -1, 1}, {1, 0, 0, -1}, {-1, 1, 0, -1},
  {0, -1, 1, 1}, {1, 1, -2, 0}, {-1, 2, -2, 0}, {0, -1, 2, -1}, {0, 0, -1, 2}, {2, -1, 0, 0}}
```

```
In[12]:= AlphaBasis[PositiveRoots[F4]]
```

```
Out[12]= {(2, 3, 4, 2), (1, 3, 4, 2), (1, 2, 4, 2), (1, 2, 3, 2), (1, 2, 3, 1), (1, 2, 2, 2), (1, 2, 2, 1), (1, 1, 2, 2),
  (0, 1, 2, 2), (1, 2, 2, 0), (1, 1, 2, 1), (0, 1, 2, 1), (1, 1, 2, 0), (1, 1, 1, 1), (0, 1, 2, 0), (0, 1, 1, 1),
  (1, 1, 1, 0), (0, 1, 1, 0), (0, 0, 1, 1), (1, 1, 0, 0), (0, 1, 0, 0), (0, 0, 1, 0), (0, 0, 0, 1), (1, 0, 0, 0)}
```

## Case $\alpha_2$

The semisimple part of the Levi factor is  $A_1 \oplus A_2$ .

The concrete identification is  $(\alpha_1) \cup (\alpha_3, \alpha_4) \leftrightarrow (\alpha_1) \cup (\alpha_1, \alpha_2)$ .

```
In[13]:= λ[1] = Weight[F4][1, -1, 0, 2];
```

```
λ[3] = Weight[F4][1, 0, 0, 0];
```

```
In[15]:= AlphaBasis[{λ[1], λ[3]}]
```

```
Out[15]= {(1, 1, 2, 2), (2, 3, 4, 2)}
```

These correspond to the highest weights  $\lambda_1 = (\omega_1, 2\omega_2)$  and  $\lambda_3 = (\omega_1, 0)$ .

```
In[16]:= V[1] = ProductIrrep[Irrep[A][1], Irrep[A][0, 2]];
```

```
In[17]:= DecomposeProduct[V[1], V[1], V[1]] // StandardForm
```

```
Out[17]//StandardForm=
```

$$2 \left( \begin{pmatrix} 1 \\ 1 \end{pmatrix}, \begin{pmatrix} 0 \\ 0 \end{pmatrix} \right) + \left( \begin{pmatrix} 3 \\ 1 \end{pmatrix}, \begin{pmatrix} 0 \\ 0 \end{pmatrix} \right) + 4 \left( \begin{pmatrix} 1 \\ 1 \end{pmatrix}, \begin{pmatrix} 1 \\ 1 \end{pmatrix} \right) + 2 \left( \begin{pmatrix} 3 \\ 1 \end{pmatrix}, \begin{pmatrix} 1 \\ 1 \end{pmatrix} \right) + \\ 2 \left( \begin{pmatrix} 1 \\ 1 \end{pmatrix}, \begin{pmatrix} 3 \\ 0 \end{pmatrix} \right) + 2 \left( \begin{pmatrix} 1 \\ 1 \end{pmatrix}, \begin{pmatrix} 0 \\ 3 \end{pmatrix} \right) + \left( \begin{pmatrix} 3 \\ 1 \end{pmatrix}, \begin{pmatrix} 3 \\ 0 \end{pmatrix} \right) + \left( \begin{pmatrix} 3 \\ 1 \end{pmatrix}, \begin{pmatrix} 0 \\ 3 \end{pmatrix} \right) + 6 \left( \begin{pmatrix} 1 \\ 1 \end{pmatrix}, \begin{pmatrix} 2 \\ 2 \end{pmatrix} \right) + \\ 2 \left( \begin{pmatrix} 1 \\ 1 \end{pmatrix}, \begin{pmatrix} 0 \\ 6 \end{pmatrix} \right) + 3 \left( \begin{pmatrix} 3 \\ 1 \end{pmatrix}, \begin{pmatrix} 2 \\ 2 \end{pmatrix} \right) + \left( \begin{pmatrix} 3 \\ 1 \end{pmatrix}, \begin{pmatrix} 0 \\ 6 \end{pmatrix} \right) + 4 \left( \begin{pmatrix} 1 \\ 1 \end{pmatrix}, \begin{pmatrix} 1 \\ 4 \end{pmatrix} \right) + 2 \left( \begin{pmatrix} 3 \\ 1 \end{pmatrix}, \begin{pmatrix} 1 \\ 4 \end{pmatrix} \right)$$

We see that  $V(\omega_1, 0)$  appears with multiplicity two.

## Case $\alpha_3$

The semisimple part of the Levi factor is  $A_2 \oplus A_1$ .

The concrete identification is  $(\alpha_1, \alpha_2) \cup (\alpha_4) \leftrightarrow (\alpha_1, \alpha_2) \cup (\alpha_1)$ .

```
In[18]:= λ[1] = Weight[F4][1, 0, -1, 1];
```

```
λ[3] = Weight[F4][0, 0, 0, 1];
```

```
In[20]:= AlphaBasis[{λ[1], λ[3]}]
```

```
Out[20]= {(1, 1, 1, 1), (1, 2, 3, 2)}
```

These correspond to the highest weights  $\lambda_1 = (\omega_1, \omega_1)$  and  $\lambda_3 = (0, \omega_1)$ .

```
In[21]:= V[1] = ProductIrrep[Irrep[A][1, 0], Irrep[A][1]];
```

```
In[22]:= DecomposeProduct[V[1], V[1], V[1]] // StandardForm
```

```
Out[22]//StandardForm=
```

$$2 \left( \begin{pmatrix} 0 \\ 0 \end{pmatrix}, \begin{pmatrix} 1 \\ 1 \end{pmatrix} \right) + \left( \begin{pmatrix} 0 \\ 0 \end{pmatrix}, \begin{pmatrix} 3 \\ 1 \end{pmatrix} \right) + 4 \left( \begin{pmatrix} 1 \\ 1 \end{pmatrix}, \begin{pmatrix} 1 \\ 1 \end{pmatrix} \right) + 2 \left( \begin{pmatrix} 3 \\ 1 \end{pmatrix}, \begin{pmatrix} 1 \\ 1 \end{pmatrix} \right) + 2 \left( \begin{pmatrix} 1 \\ 1 \end{pmatrix}, \begin{pmatrix} 3 \\ 1 \end{pmatrix} \right) + \left( \begin{pmatrix} 3 \\ 1 \end{pmatrix}, \begin{pmatrix} 3 \\ 1 \end{pmatrix} \right)$$

We see that  $V(0, \omega_1)$  appears with multiplicity two.

## Case $E_6$

```
In[83]:= DynkinDiagram[E6]
```

```
Out[83]=
```

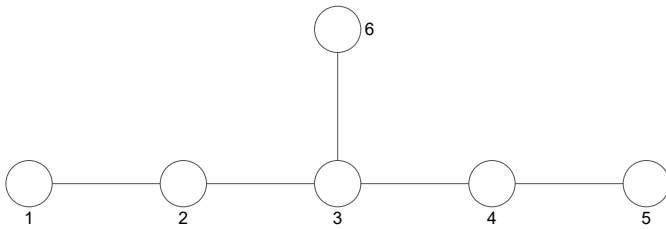

```
In[23]:= AlphaBasis[HighestRoot[E6]]
```

```
Out[23]= (1, 2, 3, 2, 1, 2)
```

In[24]:= **PositiveRoots[E6]**

Out[24]= {  $\begin{bmatrix} 0 & 0 & 0 & 0 & 0 & 1 \end{bmatrix}$ ,  $\begin{bmatrix} 0 & 0 & 1 & 0 & 0 & -1 \end{bmatrix}$ ,  $\begin{bmatrix} 0 & 1 & -1 & 1 & 0 & 0 \end{bmatrix}$ ,  $\begin{bmatrix} 0 & 1 & 0 & -1 & 1 & 0 \end{bmatrix}$ ,  $\begin{bmatrix} 1 & -1 & 0 & 1 & 0 & 0 \end{bmatrix}$ ,  
 $\begin{bmatrix} -1 & 0 & 0 & 1 & 0 & 0 \end{bmatrix}$ ,  $\begin{bmatrix} 0 & 1 & 0 & 0 & -1 & 0 \end{bmatrix}$ ,  $\begin{bmatrix} 1 & -1 & 1 & -1 & 1 & 0 \end{bmatrix}$ ,  $\begin{bmatrix} -1 & 0 & 1 & -1 & 1 & 0 \end{bmatrix}$ ,  $\begin{bmatrix} 1 & -1 & 1 & 0 & -1 & 0 \end{bmatrix}$ ,  
 $\begin{bmatrix} 1 & 0 & -1 & 0 & 1 & 1 \end{bmatrix}$ ,  $\begin{bmatrix} -1 & 0 & 1 & 0 & -1 & 0 \end{bmatrix}$ ,  $\begin{bmatrix} -1 & 1 & -1 & 0 & 1 & 1 \end{bmatrix}$ ,  $\begin{bmatrix} 1 & 0 & -1 & 1 & -1 & 1 \end{bmatrix}$ ,  $\begin{bmatrix} 1 & 0 & 0 & 0 & 1 & -1 \end{bmatrix}$ ,  
 $\begin{bmatrix} -1 & 1 & -1 & 1 & -1 & 1 \end{bmatrix}$ ,  $\begin{bmatrix} -1 & 1 & 0 & 0 & 1 & -1 \end{bmatrix}$ ,  $\begin{bmatrix} 0 & -1 & 0 & 0 & 1 & 1 \end{bmatrix}$ ,  $\begin{bmatrix} 1 & 0 & 0 & -1 & 0 & 1 \end{bmatrix}$ ,  
 $\begin{bmatrix} 1 & 0 & 0 & 1 & -1 & -1 \end{bmatrix}$ ,  $\begin{bmatrix} -1 & 1 & 0 & -1 & 0 & 1 \end{bmatrix}$ ,  $\begin{bmatrix} -1 & 1 & 0 & 1 & -1 & -1 \end{bmatrix}$ ,  $\begin{bmatrix} 0 & -1 & 0 & 1 & -1 & 1 \end{bmatrix}$ ,  
 $\begin{bmatrix} 0 & -1 & 1 & 0 & 1 & -1 \end{bmatrix}$ ,  $\begin{bmatrix} 1 & 0 & 1 & -1 & 0 & -1 \end{bmatrix}$ ,  $\begin{bmatrix} -1 & 1 & 1 & -1 & 0 & -1 \end{bmatrix}$ ,  $\begin{bmatrix} 0 & -1 & 1 & -1 & 0 & 1 \end{bmatrix}$ ,  
 $\begin{bmatrix} 0 & -1 & 1 & 1 & -1 & -1 \end{bmatrix}$ ,  $\begin{bmatrix} 0 & 0 & -1 & 1 & 1 & 0 \end{bmatrix}$ ,  $\begin{bmatrix} 1 & 1 & -1 & 0 & 0 & 0 \end{bmatrix}$ ,  $\begin{bmatrix} -1 & 2 & -1 & 0 & 0 & 0 \end{bmatrix}$ ,  
 $\begin{bmatrix} 0 & -1 & 2 & -1 & 0 & -1 \end{bmatrix}$ ,  $\begin{bmatrix} 0 & 0 & -1 & 0 & 0 & 2 \end{bmatrix}$ ,  $\begin{bmatrix} 0 & 0 & -1 & 2 & -1 & 0 \end{bmatrix}$ ,  $\begin{bmatrix} 0 & 0 & 0 & -1 & 2 & 0 \end{bmatrix}$ ,  $\begin{bmatrix} 2 & -1 & 0 & 0 & 0 & 0 \end{bmatrix}$  }

In[25]:= **AlphaBasis[PositiveRoots[E6]]**

Out[25]= {(1, 2, 3, 2, 1, 2), (1, 2, 3, 2, 1, 1), (1, 2, 2, 2, 1, 1), (1, 2, 2, 1, 1, 1), (1, 1, 2, 2, 1, 1), (0, 1, 2, 2, 1, 1),  
(1, 2, 2, 1, 0, 1), (1, 1, 2, 1, 1, 1), (0, 1, 2, 1, 1, 1), (1, 1, 2, 1, 0, 1), (1, 1, 1, 1, 1, 1), (0, 1, 2, 1, 0, 1),  
(0, 1, 1, 1, 1, 1), (1, 1, 1, 1, 0, 1), (1, 1, 1, 1, 1, 0), (0, 1, 1, 1, 0, 1), (0, 1, 1, 1, 1, 0), (0, 0, 1, 1, 1, 1),  
(1, 1, 1, 0, 0, 1), (1, 1, 1, 1, 0, 0), (0, 1, 1, 0, 0, 1), (0, 1, 1, 1, 0, 0), (0, 0, 1, 1, 0, 1), (0, 0, 1, 1, 1, 0),  
(1, 1, 1, 0, 0, 0), (0, 1, 1, 0, 0, 0), (0, 0, 1, 0, 0, 1), (0, 0, 1, 1, 0, 0), (0, 0, 0, 1, 1, 0), (1, 1, 0, 0, 0, 0),  
(0, 1, 0, 0, 0, 0), (0, 0, 1, 0, 0, 0), (0, 0, 0, 0, 0, 1), (0, 0, 0, 1, 0, 0), (0, 0, 0, 0, 1, 0), (1, 0, 0, 0, 0, 0)}

## Case $\alpha_3$

The semisimple part of the Levi factor is  $A_2 \oplus A_2 \oplus A_1$ .

The concrete identification is  $(\alpha_1, \alpha_2) \cup (\alpha_4, \alpha_5) \cup (\alpha_6) \leftrightarrow (\alpha_1, \alpha_2) \cup (\alpha_1, \alpha_2) \cup (\alpha_1)$ .

In[26]:=  $\lambda[1] = \text{Weight}[E6][1, 0, -1, 0, 1, 1];$   
 $\lambda[3] = \text{Weight}[E6][0, 0, 0, 0, 0, 1];$

In[28]:= **AlphaBasis[{ $\lambda[1]$ ,  $\lambda[3]$ }]**

Out[28]= {(1, 1, 1, 1, 1, 1), (1, 2, 3, 2, 1, 2)}

These correspond to the highest weights  $\lambda_1 = (\omega_1, \omega_2, \omega_1)$  and  $\lambda_3 = (0, 0, \omega_1)$ .

In[29]:= **V[1] = ProductIrrep[Irrep[A][1, 0], Irrep[A][0, 1], Irrep[A][1]];**

In[30]:= **DecomposeProduct[V[1], V[1], V[1]] // StandardForm**

Out[30]//StandardForm=

$$2 \left( (00), (00), (1) \right) + \left( (00), (00), (3) \right) + 4 \left( (11), (00), (1) \right) +$$

$$4 \left( (00), (11), (1) \right) + 2 \left( (30), (00), (1) \right) + 2 \left( (11), (00), (3) \right) +$$

$$2 \left( (00), (11), (3) \right) + 2 \left( (00), (03), (1) \right) + \left( (30), (00), (3) \right) + \left( (00), (03), (3) \right) +$$

$$8 \left( (11), (11), (1) \right) + 4 \left( (30), (11), (1) \right) + 4 \left( (11), (11), (3) \right) + 4 \left( (11), (03), (1) \right) +$$

$$2 \left( (30), (11), (3) \right) + 2 \left( (30), (03), (1) \right) + 2 \left( (11), (03), (3) \right) + \left( (30), (03), (3) \right)$$

We see that  $V(0, 0, \omega_1)$  appears with multiplicity two.

## Case $E_7$

In[84]:= **DynkinDiagram[E7]**

Out[84]=

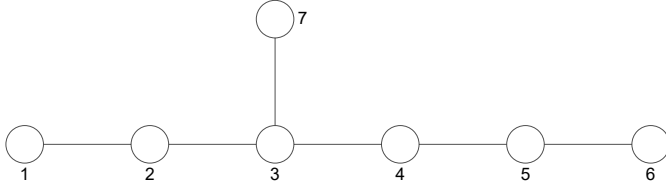

In[31]:= **AlphaBasis[HighestRoot[E7]]**

Out[31]= (2, 3, 4, 3, 2, 1, 2)

In[32]:= **PositiveRoots[E7]**

Out[32]= {  
 $\begin{bmatrix} 1 & 0 & 0 & 0 & 0 & 0 & 0 \end{bmatrix}$ ,  $\begin{bmatrix} -1 & 1 & 0 & 0 & 0 & 0 & 0 \end{bmatrix}$ ,  $\begin{bmatrix} 0 & -1 & 1 & 0 & 0 & 0 & 0 \end{bmatrix}$ ,  $\begin{bmatrix} 0 & 0 & -1 & 1 & 0 & 0 & 1 \end{bmatrix}$ ,  
 $\begin{bmatrix} 0 & 0 & 0 & -1 & 1 & 0 & 1 \end{bmatrix}$ ,  $\begin{bmatrix} 0 & 0 & 0 & 1 & 0 & 0 & -1 \end{bmatrix}$ ,  $\begin{bmatrix} 0 & 0 & 0 & 0 & -1 & 1 & 1 \end{bmatrix}$ ,  $\begin{bmatrix} 0 & 0 & 1 & -1 & 1 & 0 & -1 \end{bmatrix}$ ,  
 $\begin{bmatrix} 0 & 0 & 0 & 0 & 0 & -1 & 1 \end{bmatrix}$ ,  $\begin{bmatrix} 0 & 0 & 1 & 0 & -1 & 1 & -1 \end{bmatrix}$ ,  $\begin{bmatrix} 0 & 1 & -1 & 0 & 1 & 0 & 0 \end{bmatrix}$ ,  $\begin{bmatrix} 0 & 0 & 1 & 0 & 0 & -1 & -1 \end{bmatrix}$ ,  
 $\begin{bmatrix} 0 & 1 & -1 & 1 & -1 & 1 & 0 \end{bmatrix}$ ,  $\begin{bmatrix} 1 & -1 & 0 & 0 & 1 & 0 & 0 \end{bmatrix}$ ,  $\begin{bmatrix} -1 & 0 & 0 & 0 & 1 & 0 & 0 \end{bmatrix}$ ,  $\begin{bmatrix} 0 & 1 & -1 & 1 & 0 & -1 & 0 \end{bmatrix}$ ,  
 $\begin{bmatrix} 0 & 1 & 0 & -1 & 0 & 1 & 0 \end{bmatrix}$ ,  $\begin{bmatrix} 1 & -1 & 0 & 1 & -1 & 1 & 0 \end{bmatrix}$ ,  $\begin{bmatrix} -1 & 0 & 0 & 1 & -1 & 1 & 0 \end{bmatrix}$ ,  $\begin{bmatrix} 0 & 1 & 0 & -1 & 1 & -1 & 0 \end{bmatrix}$ ,  
 $\begin{bmatrix} 1 & -1 & 0 & 1 & 0 & -1 & 0 \end{bmatrix}$ ,  $\begin{bmatrix} 1 & -1 & 1 & -1 & 0 & 1 & 0 \end{bmatrix}$ ,  $\begin{bmatrix} -1 & 0 & 0 & 1 & 0 & -1 & 0 \end{bmatrix}$ ,  $\begin{bmatrix} -1 & 0 & 1 & -1 & 0 & 1 & 0 \end{bmatrix}$ ,  
 $\begin{bmatrix} 0 & 1 & 0 & 0 & -1 & 0 & 0 \end{bmatrix}$ ,  $\begin{bmatrix} 1 & -1 & 1 & -1 & 1 & -1 & 0 \end{bmatrix}$ ,  $\begin{bmatrix} 1 & 0 & -1 & 0 & 0 & 1 & 1 \end{bmatrix}$ ,  $\begin{bmatrix} -1 & 0 & 1 & -1 & 1 & -1 & 0 \end{bmatrix}$ ,  
 $\begin{bmatrix} -1 & 1 & -1 & 0 & 0 & 1 & 1 \end{bmatrix}$ ,  $\begin{bmatrix} 1 & -1 & 1 & 0 & -1 & 0 & 0 \end{bmatrix}$ ,  $\begin{bmatrix} 1 & 0 & -1 & 0 & 1 & -1 & 1 \end{bmatrix}$ ,  $\begin{bmatrix} 1 & 0 & 0 & 0 & 0 & 1 & -1 \end{bmatrix}$ ,  
 $\begin{bmatrix} -1 & 0 & 1 & 0 & -1 & 0 & 0 \end{bmatrix}$ ,  $\begin{bmatrix} -1 & 1 & -1 & 0 & 1 & -1 & 1 \end{bmatrix}$ ,  $\begin{bmatrix} -1 & 1 & 0 & 0 & 0 & 1 & -1 \end{bmatrix}$ ,  
 $\begin{bmatrix} 0 & -1 & 0 & 0 & 0 & 1 & 1 \end{bmatrix}$ ,  $\begin{bmatrix} 1 & 0 & -1 & 1 & -1 & 0 & 1 \end{bmatrix}$ ,  $\begin{bmatrix} 1 & 0 & 0 & 0 & 1 & -1 & -1 \end{bmatrix}$ ,  $\begin{bmatrix} -1 & 1 & -1 & 1 & -1 & 0 & 1 \end{bmatrix}$ ,  
 $\begin{bmatrix} -1 & 1 & 0 & 0 & 1 & -1 & -1 \end{bmatrix}$ ,  $\begin{bmatrix} 0 & -1 & 0 & 0 & 1 & -1 & 1 \end{bmatrix}$ ,  $\begin{bmatrix} 0 & -1 & 1 & 0 & 0 & 1 & -1 \end{bmatrix}$ ,  $\begin{bmatrix} 1 & 0 & 0 & -1 & 0 & 0 & 1 \end{bmatrix}$ ,  
 $\begin{bmatrix} 1 & 0 & 0 & 1 & -1 & 0 & -1 \end{bmatrix}$ ,  $\begin{bmatrix} -1 & 1 & 0 & -1 & 0 & 0 & 1 \end{bmatrix}$ ,  $\begin{bmatrix} -1 & 1 & 0 & 1 & -1 & 0 & -1 \end{bmatrix}$ ,  $\begin{bmatrix} 0 & -1 & 0 & 1 & -1 & 0 & 1 \end{bmatrix}$ ,  
 $\begin{bmatrix} 0 & -1 & 1 & 0 & 1 & -1 & -1 \end{bmatrix}$ ,  $\begin{bmatrix} 0 & 0 & -1 & 1 & 0 & 1 & 0 \end{bmatrix}$ ,  $\begin{bmatrix} 1 & 0 & 1 & -1 & 0 & 0 & -1 \end{bmatrix}$ ,  $\begin{bmatrix} -1 & 1 & 1 & -1 & 0 & 0 & -1 \end{bmatrix}$ ,  
 $\begin{bmatrix} 0 & -1 & 1 & -1 & 0 & 0 & 1 \end{bmatrix}$ ,  $\begin{bmatrix} 0 & -1 & 1 & 1 & -1 & 0 & -1 \end{bmatrix}$ ,  $\begin{bmatrix} 0 & 0 & -1 & 1 & 1 & -1 & 0 \end{bmatrix}$ ,  $\begin{bmatrix} 0 & 0 & 0 & -1 & 1 & 1 & 0 \end{bmatrix}$ ,  
 $\begin{bmatrix} 1 & 1 & -1 & 0 & 0 & 0 & 0 \end{bmatrix}$ ,  $\begin{bmatrix} -1 & 2 & -1 & 0 & 0 & 0 & 0 \end{bmatrix}$ ,  $\begin{bmatrix} 0 & -1 & 2 & -1 & 0 & 0 & -1 \end{bmatrix}$ ,  $\begin{bmatrix} 0 & 0 & -1 & 0 & 0 & 0 & 2 \end{bmatrix}$ ,  
 $\begin{bmatrix} 0 & 0 & -1 & 2 & -1 & 0 & 0 \end{bmatrix}$ ,  $\begin{bmatrix} 0 & 0 & 0 & -1 & 2 & -1 & 0 \end{bmatrix}$ ,  $\begin{bmatrix} 0 & 0 & 0 & 0 & -1 & 2 & 0 \end{bmatrix}$ ,  $\begin{bmatrix} 2 & -1 & 0 & 0 & 0 & 0 & 0 \end{bmatrix}$ }

```
In[33]:= AlphaBasis[PositiveRoots[E7]]
```

```
Out[33]= {(2, 3, 4, 3, 2, 1, 2), (1, 3, 4, 3, 2, 1, 2), (1, 2, 4, 3, 2, 1, 2), (1, 2, 3, 3, 2, 1, 2), (1, 2, 3, 2, 2, 1, 2), (1, 2, 3, 3, 2, 1, 1),
(1, 2, 3, 2, 1, 1, 2), (1, 2, 3, 2, 2, 1, 1), (1, 2, 3, 2, 1, 0, 2), (1, 2, 3, 2, 1, 1, 1), (1, 2, 2, 2, 2, 1, 1), (1, 2, 3, 2, 1, 0, 1),
(1, 2, 2, 2, 1, 1, 1), (1, 1, 2, 2, 2, 1, 1), (0, 1, 2, 2, 2, 1, 1), (1, 2, 2, 2, 1, 0, 1), (1, 2, 2, 1, 1, 1, 1), (1, 1, 2, 2, 1, 1, 1),
(0, 1, 2, 2, 1, 1, 1), (1, 2, 2, 1, 1, 0, 1), (1, 1, 2, 2, 1, 0, 1), (1, 1, 2, 1, 1, 1, 1), (0, 1, 2, 2, 1, 0, 1), (0, 1, 2, 1, 1, 1, 1),
(1, 2, 2, 1, 0, 0, 1), (1, 1, 2, 1, 1, 0, 1), (1, 1, 1, 1, 1, 1, 1), (0, 1, 2, 1, 1, 0, 1), (0, 1, 1, 1, 1, 1, 1), (1, 1, 2, 1, 0, 0, 1),
(1, 1, 1, 1, 1, 0, 1), (1, 1, 1, 1, 1, 1, 0), (0, 1, 2, 1, 0, 0, 1), (0, 1, 1, 1, 1, 0, 1), (0, 1, 1, 1, 1, 1, 0), (0, 0, 1, 1, 1, 1, 1),
(1, 1, 1, 1, 0, 0, 1), (1, 1, 1, 1, 1, 0, 0), (0, 1, 1, 1, 0, 0, 1), (0, 1, 1, 1, 1, 0, 0), (0, 0, 1, 1, 1, 0, 1), (0, 0, 1, 1, 1, 1, 0),
(1, 1, 1, 0, 0, 0, 1), (1, 1, 1, 1, 0, 0, 0), (0, 1, 1, 0, 0, 0, 1), (0, 1, 1, 1, 0, 0, 0), (0, 0, 1, 1, 0, 0, 1), (0, 0, 1, 1, 1, 0, 0),
(0, 0, 0, 1, 1, 1, 0), (1, 1, 1, 0, 0, 0, 0), (0, 1, 1, 0, 0, 0, 0), (0, 0, 1, 0, 0, 0, 1), (0, 0, 1, 1, 0, 0, 0),
(0, 0, 0, 1, 1, 0, 0), (0, 0, 0, 0, 1, 1, 0), (1, 1, 0, 0, 0, 0, 0), (0, 1, 0, 0, 0, 0, 0), (0, 0, 1, 0, 0, 0, 0),
(0, 0, 0, 0, 0, 0, 1), (0, 0, 0, 1, 0, 0, 0), (0, 0, 0, 0, 1, 0, 0), (0, 0, 0, 0, 0, 1, 0), (1, 0, 0, 0, 0, 0, 0)}
```

## Case $\alpha_2$

The semisimple part of the Levi factor is  $A_1 \oplus A_5$ .

The concrete identification is  $(\alpha_1) \cup (\alpha_7, \alpha_3, \alpha_4, \alpha_5, \alpha_6) \leftrightarrow (\alpha_1) \cup (\alpha_1, \alpha_2, \alpha_3, \alpha_4, \alpha_5)$ .

```
In[34]:= λ[1] = Weight[E7][1, -1, 0, 0, 1, 0, 0];
λ[3] = Weight[E7][1, 0, 0, 0, 0, 0, 0];
```

```
In[36]:= AlphaBasis[{λ[1], λ[3]}]
```

```
Out[36]= {(1, 1, 2, 2, 2, 1, 1), (2, 3, 4, 3, 2, 1, 2)}
```

These correspond to the highest weights  $\lambda_1 = (\omega_1, \omega_4)$  and  $\lambda_3 = (\omega_1, 0)$ .

```
In[37]:= V[1] = ProductIrrep[Irrep[A][1], Irrep[A][0, 0, 0, 1, 0]];
```

```
In[38]:= DecomposeProduct[V[1], V[1], V[1]] // StandardForm
```

```
Out[38]//StandardForm=
2 ((1), (00000)) + ((3), (00000)) + 4 ((1), (10001)) + 2 ((3), (10001)) + 2 ((1), (00200)) +
((3), (00200)) + 6 ((1), (01010)) + 3 ((3), (01010)) + 2 ((1), (01002)) +
((3), (01002)) + 2 ((1), (00030)) + ((3), (00030)) + 4 ((1), (00111)) + 2 ((3), (00111))
```

We see that  $V(\omega_1, 0)$  appears with multiplicity two.

## Case $\alpha_3$

The semisimple part of the Levi factor is  $A_2 \oplus A_3 \oplus A_1$ .

The concrete identification is  $(\alpha_1, \alpha_2) \cup (\alpha_4, \alpha_5, \alpha_6) \cup (\alpha_7) \leftrightarrow (\alpha_1, \alpha_2) \cup (\alpha_1, \alpha_2, \alpha_3) \cup (\alpha_1)$ .

```
In[39]:= λ[1] = Weight[E7][1, 0, -1, 0, 0, 1, 1];
λ[3] = Weight[E7][0, 0, -1, 1, 0, 0, 1];
```

```
In[41]:= AlphaBasis[{λ[1], λ[3]}]
```

```
Out[41]= {(1, 1, 1, 1, 1, 1, 1), (1, 2, 3, 3, 2, 1, 2)}
```

These correspond to the highest weights  $\lambda_1 = (\omega_1, \omega_3, \omega_1)$  and  $\lambda_3 = (0, \omega_1, \omega_1)$ .

```
In[42]:= V[1] = ProductIrrep[Irrep[A][1, 0], Irrep[A][0, 0, 1], Irrep[A][1]];
```

```
In[43]:= DecomposeProduct[V[1], V[1], V[1]] // StandardForm
```

```
Out[43]//StandardForm=
```

$$\begin{aligned}
& 2 \left( (00), (100), (1) \right) + \left( (00), (100), (3) \right) + 4 \left( (11), (100), (1) \right) + \\
& 2 \left( (30), (100), (1) \right) + 2 \left( (11), (100), (3) \right) + \left( (30), (100), (3) \right) + 4 \left( (00), (011), (1) \right) + \\
& 2 \left( (00), (003), (1) \right) + 2 \left( (00), (011), (3) \right) + \left( (00), (003), (3) \right) + 8 \left( (11), (011), (1) \right) + \\
& 4 \left( (11), (003), (1) \right) + 4 \left( (30), (011), (1) \right) + 4 \left( (11), (011), (3) \right) + \\
& 2 \left( (30), (003), (1) \right) + 2 \left( (11), (003), (3) \right) + 2 \left( (30), (011), (3) \right) + \left( (30), (003), (3) \right)
\end{aligned}$$

We see that  $V(0, \omega_1, \omega_1)$  appears with multiplicity two.

## Case $\alpha_4$

The semisimple part of the Levi factor is  $A_4 \oplus A_2$ .

The concrete identification is  $(\alpha_1, \alpha_2, \alpha_3, \alpha_7) \cup (\alpha_5, \alpha_6) \leftrightarrow (\alpha_1, \alpha_2, \alpha_3, \alpha_4) \cup (\alpha_1, \alpha_2)$ .

```
In[44]:= λ[1] = Weight[E7][0, 1, 0, -1, 0, 1, 0];
```

```
λ[3] = Weight[E7][1, 0, 0, 0, 0, 0, 0];
```

```
In[46]:= AlphaBasis[{λ[1], λ[3]}]
```

```
Out[46]= {(1, 2, 2, 1, 1, 1, 1), (2, 3, 4, 3, 2, 1, 2)}
```

These correspond to the highest weights  $\lambda_1 = (\omega_2, \omega_2)$  and  $\lambda_3 = (\omega_1, 0)$ .

```
In[47]:= V[1] = ProductIrrep[Irrep[A][0, 1, 0, 0], Irrep[A][0, 1]];
```

```
In[48]:= DecomposeProduct[V[1], V[1], V[1]] // StandardForm
```

```
Out[48]//StandardForm=
```

$$\begin{aligned}
& 2 \left( (1000), (00) \right) + 4 \left( (1000), (11) \right) + 2 \left( (1000), (03) \right) + 3 \left( (0101), (00) \right) + \\
& \left( (0020), (00) \right) + 6 \left( (0101), (11) \right) + 3 \left( (0101), (03) \right) + 2 \left( (0020), (11) \right) + \\
& \left( (0020), (03) \right) + \left( (2001), (00) \right) + 2 \left( (2001), (11) \right) + \left( (2001), (03) \right) + \left( (0300), (00) \right) + \\
& 2 \left( (0300), (11) \right) + \left( (0300), (03) \right) + 2 \left( (1110), (00) \right) + 4 \left( (1110), (11) \right) + 2 \left( (1110), (03) \right)
\end{aligned}$$

We see that  $V(\omega_1, 0)$  appears with multiplicity two.

## Case $E_8$

```
In[85]:= DynkinDiagram[E8]
```

```
Out[85]=
```

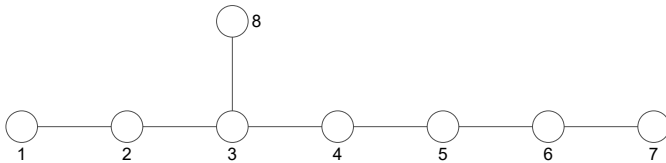

```
In[49]:= AlphaBasis[HighestRoot[E8]]
```

```
Out[49]= (2, 4, 6, 5, 4, 3, 2, 3)
```

```
In[50]:= PositiveRoots[E8]
```

```
Out[50]= { [0 0 0 0 0 0 1 0], [0 0 0 0 0 1 -1 0], [0 0 0 0 1 -1 0 0], [0 0 0 1 -1 0 0 0],
            [0 0 1 -1 0 0 0 0], [0 1 -1 0 0 0 0 1], [0 1 0 0 0 0 0 -1], [1 -1 0 0 0 0 0 1],
```

$[-1\ 0\ 0\ 0\ 0\ 0\ 0\ 1], [-1\ 1\ 0\ 0\ 0\ 0\ 0\ -1], [-1\ 0\ 1\ 0\ 0\ 0\ 0\ -1], [1\ 0\ -1\ 1\ 0\ 0\ 0\ 0],$   
 $[-1\ 1\ -1\ 1\ 0\ 0\ 0\ 0], [1\ 0\ 0\ -1\ 1\ 0\ 0\ 0], [-1\ 1\ 0\ -1\ 1\ 0\ 0\ 0], [0\ -1\ 0\ 1\ 0\ 0\ 0\ 0],$   
 $[1\ 0\ 0\ 0\ -1\ 1\ 0\ 0], [-1\ 1\ 0\ 0\ -1\ 1\ 0\ 0], [0\ -1\ 1\ -1\ 1\ 0\ 0\ 0], [1\ 0\ 0\ 0\ 0\ -1\ 1\ 0],$   
 $[-1\ 1\ 0\ 0\ 0\ -1\ 1\ 0], [0\ -1\ 1\ 0\ -1\ 1\ 0\ 0], [0\ 0\ -1\ 0\ 1\ 0\ 0\ 1], [1\ 0\ 0\ 0\ 0\ 0\ -1\ 0],$   
 $[-1\ 1\ 0\ 0\ 0\ 0\ -1\ 0], [0\ -1\ 1\ 0\ 0\ -1\ 1\ 0], [0\ 0\ -1\ 1\ -1\ 1\ 0\ 1], [0\ 0\ 0\ 0\ 1\ 0\ 0\ -1],$   
 $[0\ -1\ 1\ 0\ 0\ 0\ -1\ 0], [0\ 0\ -1\ 1\ 0\ -1\ 1\ 1], [0\ 0\ 0\ -1\ 0\ 1\ 0\ 1], [0\ 0\ 0\ 1\ -1\ 1\ 0\ -1],$   
 $[0\ 0\ -1\ 1\ 0\ 0\ -1\ 1], [0\ 0\ 0\ -1\ 1\ -1\ 1\ 1], [0\ 0\ 0\ 1\ 0\ -1\ 1\ -1],$   
 $[0\ 0\ 1\ -1\ 0\ 1\ 0\ -1], [0\ 0\ 0\ -1\ 1\ 0\ -1\ 1], [0\ 0\ 0\ 0\ -1\ 0\ 1\ 1], [0\ 0\ 0\ 1\ 0\ 0\ -1\ -1],$   
 $[0\ 0\ 1\ -1\ 1\ -1\ 1\ -1], [0\ 1\ -1\ 0\ 0\ 1\ 0\ 0], [0\ 0\ 0\ 0\ -1\ 1\ -1\ 1],$   
 $[0\ 0\ 1\ -1\ 1\ 0\ -1\ -1], [0\ 0\ 1\ 0\ -1\ 0\ 1\ -1], [0\ 1\ -1\ 0\ 1\ -1\ 1\ 0],$   
 $[1\ -1\ 0\ 0\ 0\ 1\ 0\ 0], [-1\ 0\ 0\ 0\ 0\ 1\ 0\ 0], [0\ 0\ 0\ 0\ 0\ -1\ 0\ 1], [0\ 0\ 1\ 0\ -1\ 1\ -1\ -1],$   
 $[0\ 1\ -1\ 0\ 1\ 0\ -1\ 0], [0\ 1\ -1\ 1\ -1\ 0\ 1\ 0], [1\ -1\ 0\ 0\ 1\ -1\ 1\ 0],$   
 $[-1\ 0\ 0\ 0\ 1\ -1\ 1\ 0], [0\ 0\ 1\ 0\ 0\ -1\ 0\ -1], [0\ 1\ -1\ 1\ -1\ 1\ -1\ 0],$   
 $[0\ 1\ 0\ -1\ 0\ 0\ 1\ 0], [1\ -1\ 0\ 0\ 1\ 0\ -1\ 0], [1\ -1\ 0\ 1\ -1\ 0\ 1\ 0], [-1\ 0\ 0\ 0\ 1\ 0\ -1\ 0],$   
 $[-1\ 0\ 0\ 1\ -1\ 0\ 1\ 0], [0\ 1\ -1\ 1\ 0\ -1\ 0\ 0], [0\ 1\ 0\ -1\ 0\ 1\ -1\ 0],$   
 $[1\ -1\ 0\ 1\ -1\ 1\ -1\ 0], [1\ -1\ 1\ -1\ 0\ 0\ 1\ 0], [-1\ 0\ 0\ 1\ -1\ 1\ -1\ 0],$   
 $[-1\ 0\ 1\ -1\ 0\ 0\ 1\ 0], [0\ 1\ 0\ -1\ 1\ -1\ 0\ 0], [1\ -1\ 0\ 1\ 0\ -1\ 0\ 0],$   
 $[1\ -1\ 1\ -1\ 0\ 1\ -1\ 0], [1\ 0\ -1\ 0\ 0\ 0\ 1\ 1], [-1\ 0\ 0\ 1\ 0\ -1\ 0\ 0],$   
 $[-1\ 0\ 1\ -1\ 0\ 1\ -1\ 0], [-1\ 1\ -1\ 0\ 0\ 0\ 1\ 1], [0\ 1\ 0\ 0\ -1\ 0\ 0\ 0],$   
 $[1\ -1\ 1\ -1\ 1\ -1\ 0\ 0], [1\ 0\ -1\ 0\ 0\ 1\ -1\ 1], [1\ 0\ 0\ 0\ 0\ 0\ 1\ -1],$   
 $[-1\ 0\ 1\ -1\ 1\ -1\ 0\ 0], [-1\ 1\ -1\ 0\ 0\ 1\ -1\ 1], [-1\ 1\ 0\ 0\ 0\ 0\ 1\ -1],$   
 $[0\ -1\ 0\ 0\ 0\ 0\ 1\ 1], [1\ -1\ 1\ 0\ -1\ 0\ 0\ 0], [1\ 0\ -1\ 0\ 1\ -1\ 0\ 1], [1\ 0\ 0\ 0\ 0\ 1\ -1\ -1],$   
 $[-1\ 0\ 1\ 0\ -1\ 0\ 0\ 0], [-1\ 1\ -1\ 0\ 1\ -1\ 0\ 1], [-1\ 1\ 0\ 0\ 0\ 1\ -1\ -1],$   
 $[0\ -1\ 0\ 0\ 0\ 1\ -1\ 1], [0\ -1\ 1\ 0\ 0\ 0\ 1\ -1], [1\ 0\ -1\ 1\ -1\ 0\ 0\ 1],$   
 $[1\ 0\ 0\ 0\ 1\ -1\ 0\ -1], [-1\ 1\ -1\ 1\ -1\ 0\ 0\ 1], [-1\ 1\ 0\ 0\ 1\ -1\ 0\ -1],$   
 $[0\ -1\ 0\ 0\ 1\ -1\ 0\ 1], [0\ -1\ 1\ 0\ 0\ 1\ -1\ -1], [0\ 0\ -1\ 1\ 0\ 0\ 1\ 0], [1\ 0\ 0\ -1\ 0\ 0\ 0\ 1],$   
 $[1\ 0\ 0\ 1\ -1\ 0\ 0\ -1], [-1\ 1\ 0\ -1\ 0\ 0\ 0\ 1], [-1\ 1\ 0\ 1\ -1\ 0\ 0\ -1],$   
 $[0\ -1\ 0\ 1\ -1\ 0\ 0\ 1], [0\ -1\ 1\ 0\ 1\ -1\ 0\ -1], [0\ 0\ -1\ 1\ 0\ 1\ -1\ 0],$   
 $[0\ 0\ 0\ -1\ 1\ 0\ 1\ 0], [1\ 0\ 1\ -1\ 0\ 0\ 0\ -1], [-1\ 1\ 1\ -1\ 0\ 0\ 0\ -1],$   
 $[0\ -1\ 1\ -1\ 0\ 0\ 0\ 1], [0\ -1\ 1\ 1\ -1\ 0\ 0\ -1], [0\ 0\ -1\ 1\ 1\ -1\ 0\ 0],$   
 $[0\ 0\ 0\ -1\ 1\ 1\ -1\ 0], [0\ 0\ 0\ 0\ -1\ 1\ 1\ 0], [1\ 1\ -1\ 0\ 0\ 0\ 0\ 0], [-1\ 2\ -1\ 0\ 0\ 0\ 0\ 0],$   
 $[0\ -1\ 2\ -1\ 0\ 0\ 0\ -1], [0\ 0\ -1\ 0\ 0\ 0\ 0\ 2], [0\ 0\ -1\ 2\ -1\ 0\ 0\ 0],$   
 $[0\ 0\ 0\ -1\ 2\ -1\ 0\ 0], [0\ 0\ 0\ 0\ -1\ 2\ -1\ 0], [0\ 0\ 0\ 0\ 0\ -1\ 2\ 0], [2\ -1\ 0\ 0\ 0\ 0\ 0\ 0]\}$

```
In[51]:= AlphaBasis[PositiveRoots[E8]]
```



```
Out[51]= {(2, 4, 6, 5, 4, 3, 2, 3), (2, 4, 6, 5, 4, 3, 1, 3), (2, 4, 6, 5, 4, 2, 1, 3), (2, 4, 6, 5, 3, 2, 1, 3), (2, 4, 6, 4, 3, 2, 1, 3),
(2, 4, 5, 4, 3, 2, 1, 3), (2, 4, 5, 4, 3, 2, 1, 2), (2, 3, 5, 4, 3, 2, 1, 3), (1, 3, 5, 4, 3, 2, 1, 3), (2, 3, 5, 4, 3, 2, 1, 2),
(1, 3, 5, 4, 3, 2, 1, 2), (2, 3, 4, 4, 3, 2, 1, 2), (1, 3, 4, 4, 3, 2, 1, 2), (2, 3, 4, 3, 3, 2, 1, 2), (1, 3, 4, 3, 3, 2, 1, 2),
(1, 2, 4, 4, 3, 2, 1, 2), (2, 3, 4, 3, 2, 2, 1, 2), (1, 3, 4, 3, 2, 2, 1, 2), (1, 2, 4, 3, 3, 2, 1, 2), (2, 3, 4, 3, 2, 1, 1, 2),
(1, 3, 4, 3, 2, 1, 1, 2), (1, 2, 4, 3, 2, 2, 1, 2), (1, 2, 3, 3, 3, 2, 1, 2), (2, 3, 4, 3, 2, 1, 0, 2), (1, 3, 4, 3, 2, 1, 0, 2),
(1, 2, 4, 3, 2, 1, 1, 2), (1, 2, 3, 3, 3, 2, 1, 2), (1, 2, 3, 3, 3, 2, 1, 1), (1, 2, 4, 3, 2, 1, 0, 2), (1, 2, 3, 3, 2, 1, 1, 2),
(1, 2, 3, 2, 2, 2, 1, 2), (1, 2, 3, 3, 2, 2, 1, 1), (1, 2, 3, 3, 2, 1, 0, 2), (1, 2, 3, 2, 2, 1, 1, 2), (1, 2, 3, 3, 2, 1, 1, 1),
(1, 2, 3, 2, 2, 2, 1, 1), (1, 2, 3, 2, 2, 1, 0, 2), (1, 2, 3, 2, 1, 1, 1, 2), (1, 2, 3, 3, 2, 1, 0, 1), (1, 2, 3, 2, 2, 1, 1, 1),
(1, 2, 2, 2, 2, 2, 1, 1), (1, 2, 3, 2, 1, 1, 0, 2), (1, 2, 3, 2, 2, 1, 0, 1), (1, 2, 3, 2, 1, 1, 1, 1), (1, 2, 2, 2, 2, 1, 1, 1),
(1, 1, 2, 2, 2, 2, 1, 1), (0, 1, 2, 2, 2, 2, 1, 1), (1, 2, 3, 2, 1, 0, 0, 2), (1, 2, 3, 2, 1, 1, 0, 1), (1, 2, 2, 2, 2, 1, 0, 1),
(1, 2, 2, 2, 1, 1, 1, 1), (1, 1, 2, 2, 2, 2, 1, 1), (0, 1, 2, 2, 2, 1, 1, 1), (1, 2, 3, 2, 1, 0, 0, 1), (1, 2, 2, 2, 1, 1, 0, 1),
(1, 2, 2, 1, 1, 1, 1, 1), (1, 1, 2, 2, 2, 1, 0, 1), (1, 1, 2, 2, 1, 1, 1, 1), (0, 1, 2, 2, 2, 1, 0, 1), (0, 1, 2, 2, 1, 1, 1, 1),
(1, 2, 2, 1, 0, 0, 1), (1, 2, 2, 1, 1, 1, 0, 1), (1, 1, 2, 2, 1, 1, 0, 1), (1, 1, 2, 1, 1, 1, 1, 1), (0, 1, 2, 2, 1, 1, 0, 1),
(0, 1, 2, 1, 1, 1, 1, 1), (1, 2, 2, 1, 1, 0, 0, 1), (1, 1, 2, 2, 1, 0, 0, 1), (1, 1, 2, 1, 1, 1, 0, 1), (1, 1, 1, 1, 1, 1, 1, 1),
(0, 1, 2, 2, 1, 0, 0, 1), (0, 1, 2, 1, 1, 1, 0, 1), (0, 1, 1, 1, 1, 1, 1, 1), (1, 2, 2, 1, 0, 0, 0, 1), (1, 1, 2, 1, 1, 0, 0, 1),
(1, 1, 1, 1, 1, 1, 0, 1), (1, 1, 1, 1, 1, 1, 1, 0), (0, 1, 2, 1, 1, 0, 0, 1), (0, 1, 1, 1, 1, 1, 0, 1), (0, 1, 1, 1, 1, 1, 1, 0),
(0, 0, 1, 1, 1, 1, 1, 1), (1, 1, 2, 1, 0, 0, 0, 1), (1, 1, 1, 1, 1, 0, 0, 1), (1, 1, 1, 1, 1, 1, 0, 0), (0, 1, 2, 1, 0, 0, 0, 1),
(0, 1, 1, 1, 1, 0, 0, 1), (0, 1, 1, 1, 1, 1, 0, 0), (0, 0, 1, 1, 1, 1, 0, 1), (0, 0, 1, 1, 1, 1, 1, 0), (1, 1, 1, 1, 0, 0, 0, 1),
(1, 1, 1, 1, 1, 0, 0, 0), (0, 1, 1, 1, 0, 0, 0, 1), (0, 1, 1, 1, 1, 0, 0, 0), (0, 0, 1, 1, 1, 0, 0, 1), (0, 0, 1, 1, 1, 1, 0, 0),
(0, 0, 0, 1, 1, 1, 1, 0), (1, 1, 1, 0, 0, 0, 0, 1), (1, 1, 1, 1, 0, 0, 0, 0), (0, 1, 1, 0, 0, 0, 0, 1), (0, 1, 1, 1, 0, 0, 0, 0),
(0, 0, 1, 1, 0, 0, 0, 1), (0, 0, 1, 1, 1, 0, 0, 0), (0, 0, 0, 1, 1, 1, 0, 0), (0, 0, 0, 1, 1, 1, 1, 0), (1, 1, 1, 0, 0, 0, 0, 0),
(0, 1, 1, 0, 0, 0, 0, 1), (0, 0, 1, 1, 0, 0, 0, 0), (0, 0, 0, 1, 1, 0, 0, 0), (0, 0, 0, 1, 1, 0, 0, 0), (0, 0, 0, 0, 1, 1, 0, 0),
(1, 1, 0, 0, 0, 0, 0, 0), (0, 1, 0, 0, 0, 0, 0, 0), (0, 0, 1, 0, 0, 0, 0, 0), (0, 0, 0, 1, 0, 0, 0, 0), (0, 0, 0, 0, 0, 0, 0, 1),
(0, 0, 0, 1, 0, 0, 0, 0), (0, 0, 0, 0, 1, 0, 0, 0), (0, 0, 0, 0, 0, 1, 0, 0), (0, 0, 0, 0, 0, 0, 1, 0), (1, 0, 0, 0, 0, 0, 0, 0)}
```

## Case $\alpha_2$

The semisimple part of the Levi factor is  $A_1 \oplus A_6$ .

The concrete identification is  $(\alpha_1) \cup (\alpha_8, \alpha_3, \alpha_4, \alpha_5, \alpha_6, \alpha_7) \leftrightarrow (\alpha_1) \cup (\alpha_1, \alpha_2, \alpha_3, \alpha_4, \alpha_5, \alpha_6)$ .

```
In[52]:= λ[1] = Weight[E8][1, -1, 0, 0, 0, 1, 0, 0];
λ[3] = Weight[E8][1, -1, 0, 0, 0, 0, 0, 1];
```

```
In[54]:= AlphaBasis[{λ[1], λ[3]}]
```

```
Out[54]= {(1, 1, 2, 2, 2, 2, 1, 1), (2, 3, 5, 4, 3, 2, 1, 3)}
```

These correspond to the highest weights  $\lambda_1 = (\omega_1, \omega_5)$  and  $\lambda_3 = (\omega_1, \omega_1)$ .

```
In[55]:= V[1] = ProductIrrep[Irrep[A][1], Irrep[A][0, 0, 0, 0, 1, 0]];
```

```
In[56]:= DecomposeProduct[V[1], V[1], V[1]] // StandardForm
```

```
Out[56]//StandardForm=
```

```
2 ( (1), (100000) ) + ( (3), (100000) ) + 4 ( (1), (010001) ) +
2 ( (3), (010001) ) + 2 ( (1), (000200) ) + ( (3), (000200) ) +
6 ( (1), (001010) ) + 3 ( (3), (001010) ) + 2 ( (1), (001002) ) + ( (3), (001002) ) +
2 ( (1), (000030) ) + ( (3), (000030) ) + 4 ( (1), (000111) ) + 2 ( (3), (000111) )
```

We see that  $V(\omega_1, \omega_1)$  appears with multiplicity two.

### Case $\alpha_3$

The semisimple part of the Levi factor is  $A_2 \oplus A_4 \oplus A_1$ .

The concrete identification is  $(\alpha_1, \alpha_2) \cup (\alpha_4, \alpha_5, \alpha_6, \alpha_7) \cup (\alpha_8) \leftrightarrow (\alpha_1, \alpha_2) \cup (\alpha_1, \alpha_2, \alpha_3, \alpha_4) \cup (\alpha_1)$ .

```
In[57]:= λ[1] = Weight[E8] [1, 0, -1, 0, 0, 0, 1, 1];
λ[3] = Weight[E8] [0, 0, -1, 0, 1, 0, 0, 1];
```

```
In[59]:= AlphaBasis[{λ[1], λ[3]}]
```

```
Out[59]= {(1, 1, 1, 1, 1, 1, 1, 1), (1, 2, 3, 3, 3, 2, 1, 2)}
```

These correspond to the highest weights  $\lambda_1 = (\omega_1, \omega_4, \omega_1)$  and  $\lambda_3 = (0, \omega_2, \omega_1)$ .

```
In[60]:= V[1] = ProductIrrep[Irrep[A] [1, 0], Irrep[A] [0, 0, 0, 1], Irrep[A] [1]];
```

```
In[61]:= DecomposeProduct[V[1], V[1], V[1]] // StandardForm
```

```
Out[61]//StandardForm=
```

```
2 ((00), (0100), (1)) + ((00), (0100), (3)) + 4 ((11), (0100), (1)) + 2 ((30), (0100), (1)) +
2 ((11), (0100), (3)) + ((30), (0100), (3)) + 2 ((00), (0003), (1)) + ((00), (0003), (3)) +
4 ((00), (0011), (1)) + 2 ((00), (0011), (3)) + 4 ((11), (0003), (1)) +
2 ((30), (0003), (1)) + 2 ((11), (0003), (3)) + ((30), (0003), (3)) +
8 ((11), (0011), (1)) + 4 ((30), (0011), (1)) + 4 ((11), (0011), (3)) + 2 ((30), (0011), (3))
```

We see that  $V(0, \omega_2, \omega_1)$  appears with multiplicity two.

### Case $\alpha_4$

The semisimple part of the Levi factor is  $A_4 \oplus A_3$ .

The concrete identification is  $(\alpha_1, \alpha_2, \alpha_3, \alpha_8) \cup (\alpha_5, \alpha_6, \alpha_7) \leftrightarrow (\alpha_1, \alpha_2, \alpha_3, \alpha_4) \cup (\alpha_1, \alpha_2, \alpha_3)$ .

```
In[62]:= λ[1] = Weight[E8] [0, 1, 0, -1, 0, 0, 1, 0];
λ[3] = Weight[E8] [1, 0, 0, -1, 1, 0, 0, 0];
```

```
In[64]:= AlphaBasis[{λ[1], λ[3]}]
```

```
Out[64]= {(1, 2, 2, 1, 1, 1, 1, 1), (2, 3, 4, 3, 3, 2, 1, 2)}
```

These correspond to the highest weights  $\lambda_1 = (\omega_2, \omega_3)$  and  $\lambda_3 = (\omega_1, \omega_1)$ .

```
In[65]:= V[1] = ProductIrrep[Irrep[A] [0, 1, 0, 0], Irrep[A] [0, 0, 1]];
```

```
In[66]:= DecomposeProduct[V[1], V[1], V[1]] // StandardForm
```

```
Out[66]//StandardForm=
```

```
2 ((1000), (100)) + 4 ((1000), (011)) + 2 ((1000), (003)) +
3 ((0101), (100)) + ((0020), (100)) + 6 ((0101), (011)) +
3 ((0101), (003)) + 2 ((0020), (011)) + ((0020), (003)) + ((2001), (100)) +
2 ((2001), (011)) + ((2001), (003)) + ((0300), (100)) + 2 ((0300), (011)) +
((0300), (003)) + 2 ((1110), (100)) + 4 ((1110), (011)) + 2 ((1110), (003))
```

We see that  $V(\omega_1, \omega_1)$  appears with multiplicity two.

## Case $\alpha_5$

The semisimple part of the Levi factor is  $D_5 \oplus A_2$ .

The concrete identification is  $(\alpha_1, \alpha_2, \alpha_3, \alpha_4, \alpha_8) \cup (\alpha_6, \alpha_7) \leftrightarrow (\alpha_1, \alpha_2, \alpha_3, \alpha_4, \alpha_5) \cup (\alpha_1, \alpha_2)$ .

```
In[67]:= λ[1] = Weight[E8][0, 0, 0, 0, -1, 0, 1, 1];
λ[3] = Weight[E8][0, 0, 0, 1, -1, 0, 0, 0];
```

These correspond to the highest weights  $\lambda_1 = (\omega_5, \omega_2)$  and  $\lambda_3 = (\omega_4, 0)$ .

```
In[69]:= V[1] = ProductIrrep[Irrep[D][0, 0, 0, 0, 1], Irrep[A][0, 1]];
```

```
In[70]:= DecomposeProduct[V[1], V[1], V[1]] // StandardForm
```

Out[70]//StandardForm=

```
2 ( (00010), (00) ) + 4 ( (00010), (11) ) + 2 ( (00010), (03) ) +
3 ( (10001), (00) ) + 6 ( (10001), (11) ) + 3 ( (10001), (03) ) + ( (01010), (00) ) +
2 ( (01010), (11) ) + ( (01010), (03) ) + ( (00003), (00) ) + 2 ( (00003), (11) ) +
( (00003), (03) ) + 2 ( (00101), (00) ) + 4 ( (00101), (11) ) + 2 ( (00101), (03) )
```

We see that  $V(\omega_4, 0)$  appears with multiplicity two.

## Case $\alpha_6$

The semisimple part of the Levi factor is  $E_6 \oplus A_1$ .

The concrete identification is  $(\alpha_1, \alpha_2, \alpha_3, \alpha_4, \alpha_5, \alpha_8) \cup (\alpha_7) \leftrightarrow (\alpha_1, \alpha_2, \alpha_3, \alpha_4, \alpha_5, \alpha_6) \cup (\alpha_1)$ .

```
In[71]:= λ[1] = Weight[E8][1, 0, 0, 0, 0, -1, 1, 0];
λ[3] = Weight[E8][0, 0, 0, 0, 0, 0, 1, 0];
```

```
In[73]:= AlphaBasis[{λ[1], λ[3]}]
```

```
Out[73]= {(2, 3, 4, 3, 2, 1, 1, 2), (2, 4, 6, 5, 4, 3, 2, 3)}
```

These correspond to the highest weights  $\lambda_1 = (\omega_1, \omega_1)$  and  $\lambda_3 = (0, \omega_1)$ .

```
In[74]:= V[1] = ProductIrrep[Irrep[E6][1, 0, 0, 0, 0, 0], Irrep[A][1]];
```

```
In[75]:= DecomposeProduct[V[1], V[1], V[1]] // StandardForm
```

Out[75]//StandardForm=

```
2 ( (000000), (1) ) + ( (000000), (3) ) + 4 ( (000001), (1) ) + 2 ( (000001), (3) ) +
6 ( (100010), (1) ) + 3 ( (100010), (3) ) + 2 ( (001000), (1) ) + ( (001000), (3) ) +
2 ( (300000), (1) ) + ( (300000), (3) ) + 4 ( (110000), (1) ) + 2 ( (110000), (3) )
```

We see that  $V(0, \omega_1)$  appears with multiplicity two.

## Case $\alpha_8$

The semisimple part of the Levi factor is  $A_7$ .

The concrete identification is  $(\alpha_1, \alpha_2, \alpha_3, \alpha_4, \alpha_5, \alpha_6, \alpha_7) \leftrightarrow (\alpha_1, \alpha_2, \alpha_3, \alpha_4, \alpha_5, \alpha_6, \alpha_7)$ .

```
In[76]:= λ[1] = Weight[E8][0, 0, 0, 0, 1, 0, 0, -1];
λ[3] = Weight[E8][0, 0, 0, 0, 0, 0, 1, 0];
```

```
In[78]:= AlphaBasis[{λ[1], λ[3]}]
```

```
Out[78]= {(1, 2, 3, 3, 3, 2, 1, 1), (2, 4, 6, 5, 4, 3, 2, 3)}
```

These correspond to the highest weights  $\lambda_1 = \omega_5$  and  $\lambda_3 = \omega_7$ .

```
In[79]:= V[1] = Irrep[A][0, 0, 0, 0, 1, 0, 0];
```

```
In[80]:= DecomposeProduct[V[1], V[1], V[1]] // StandardForm
```

```
Out[80]//StandardForm=
```

```
2 (0000001) + 3 (1000010) + (1000002) + 4 (0100100) + 2 (0011000) +
2 (0100011) + (0002001) + (0000300) + (0010020) + 3 (0010101) + 2 (0001110)
```

We see that  $V(\omega_7)$  appears with multiplicity two.
